# Supplementary material for: SafePowerGraph: Safety-aware Evaluation of Graph Neural Networks for Transmission Power Grids
Source: arXiv:2407.12421 source file (2024-07-17)
Supplement: Supplementary file 1 [file scratch.tex]

30-bus & ID           & SL       & \num{0.000004} (\num{0.000010})                            & \num{0.000006} (\num{0.000011})                            & \num{9.243440e-07}(\num{0.000001})                         & \num{1.004663e-06} (\num{2.453581e-06})                  & \num{0.000061} (\num{0.000109}) & \num{0.000085} (\num{0.000500})                             \\
&              & +SSL     & {\num{0.000003} (\num{0.000009})} & \num{0.000002} (\num{0.000006})                            & \num{1.001064e-06}(\num{0.000004})                         & \num{1.488563e-07} (\num{3.556052e-07})                  & \num{0.000064}(\num{0.000116})  & {\num{0.000115} (\num{0.000607}) } \\
& Price - sage & SL       & \num{0.034056} (\num{0.077716})                            & \num{0.033182} (\num{0.052650})                            & \num{0.016075} (\num{0.038311})                            & \num{0.102260} (\num{0.279679})                          & \num{0.002033} (\num{0.003072}) & \num{0.243444} (\num{0.360693})                             \\
&             & +SSL     & {\num{0.014256} (\num{0.036290})} & {\num{0.010716} (\num{0.024505})} & {\num{0.007457} (\num{0.033905})} & {\num{0.002239}(\num{0.003304})} & \num{0.003093} (\num{0.003930}) & \num{0.473968} (\num{0.392540})                             \\
& Line         & SL       & \num{0.000029} (\num{0.000349})                            & \num{0.000045} (\num{0.000968})                            & \num{0.000002} (\num{0.000007})                            & \num{1.461339e-06} (\num{3.053494e-06})                  & \num{0.000132} (\num{0.000474}) & \num{0.000187} (\num{0.000993})                             \\
 &            & +SSL     & \num{0.000024} (\num{0.000197})                            & \num{0.000018} (\num{0.000047})                            & \num{0.000004} (\num{0.000001})                            & \num{5.813202e-07} (\num{8.033968e-07})                  & \num{0.000126} (\num{0.000480}) & \num{0.000156} (\num{0.000849})                             
\

30-bus & ID           & SL       & \num{0.000004} (\num{0.000010})                            & \num{0.000006} (\num{0.000011})                            & \num{9.243440e-07}(\num{0.000001})                         & \num{1.004663e-06} (\num{2.453581e-06})                  & \num{0.000061} (\num{0.000109}) & \num{0.000085} (\num{0.000500})                             \\
&              & +SSL     & {\num{0.000003} (\num{0.000009})} & \num{0.000002} (\num{0.000006})                            & \num{1.001064e-06}(\num{0.000004})                         & \num{1.488563e-07} (\num{3.556052e-07})                  & \num{0.000064}(\num{0.000116})  & {\num{0.000115} (\num{0.000607}) } \\
& Price - sage & SL       & \num{0.034056} (\num{0.077716})                            & \num{0.033182} (\num{0.052650})                            & \num{0.016075} (\num{0.038311})                            & \num{0.102260} (\num{0.279679})                          & \num{0.002033} (\num{0.003072}) & \num{0.243444} (\num{0.360693})                             \\
&             & +SSL     & {\num{0.014256} (\num{0.036290})} & {\num{0.010716} (\num{0.024505})} & {\num{0.007457} (\num{0.033905})} & \num{0.002239}(\num{0.003304} & \num{0.003093} (\num{0.003930}) & \num{0.473968} (\num{0.392540})                             \\
& Line         & SL       & \num{0.000029} (\num{0.000349})                            & \num{0.000045} (\num{0.000968})                            & \num{0.000002} (\num{0.000007})                            & \num{1.461339e-06} (\num{3.053494e-06})                  & \num{0.000132} (\num{0.000474}) & \num{0.000187} (\num{0.000993})                             \\
 &            & +SSL     & \num{0.000024} (\num{0.000197})                            & \num{0.000018} (\num{0.000047})                            & \num{0.000004} (\num{0.000001})                            & \num{5.813202e-07} (\num{8.033968e-07})                  & \num{0.000126} (\num{0.000480}) & \num{0.000156} (\num{0.000849})       \\

\begin{tabular}{c|c|c|cccccc}
\toprule
Case & Var    &  Learning    & P\_gen                                                  & Q\_gen                                                   & P\_slack            & Q\_slack                                                & V                                                       & $\theta$                                                     \\ 
\midrule
118-bus & ID           & SL       & \num{0.000387} (\num{0.001152})                            & \num{0.000028} (\num{0.000079}) & \num{0.000140}(\num{0.000085}) & \num{0.000187} (\num{0.000115}) & \num{0.000208} (\num{0.000441}) & \num{0.003209} (\num{0.006585})                             \\
             & +SSL     & \textbf{\num{0.000361} (\num{0.000908})} & \num{0.000027} (\num{0.000091}) & \num{0.000040}(\num{0.000021})                                     & \num{0.000021} (\num{0.000029}) & \num{0.000658}(\num{0.001379})  & \textbf{\num{0.020197} (\num{0.112317})} \\
 & Price        & SL       & \num{} (\num{})                                                                                                                    & \num{} (\num{})                                                                                         & \num{} (\num{})                                                                                                                            & \num{} (\num{})                                                                                         & \num{} (\num{})                                                                                         & \num{} (\num{})                                                                                                                     \\
 & & sage         & +SSL     & \textbf{\num{} (\num{})}                                                                                                           & \textbf{\num{} (\num{})}                                                                                & \textbf{\num{} (\num{})}                                                                                                                   & \textbf{\num{}(\num{})}                                                                                 & \num{} (\num{})                                                                                         & \num{} (\num{})                                                                                                                     \\
& Line         & SL       & \num{0.000157} (\num{0.001153})                             & \num{0.000066} (\num{0.000620}) & \num{0.000037} (\num{0.000142})                                    & \num{0.000655} (\num{0.001639}) & \num{0.000719} (\num{0.001994}) & \num{0.001956} (\num{0.005558})                             \\
        &     & +SSL     & \num{0.000551} (\num{0.005674})                           &  & \num{0.000226} (\num{0.004566}) & \num{0.000015} (\num{0.000019})                                  &   & \num{0.000144} (\num{0.000618}) & \num{0.000250} (\num{0.000700}) & \num{0.001851} (\num{0.011665})                             
  \\ 
      
      \bottomrule                                 
\end{tabular}
